# Supplementary material for: Score matching enables causal discovery of nonlinear additive noise models
Source: arXiv:2203.04413 source file (2022-03-08)
Supplement: Supplementary file 1 [file appendix.tex]

\section{appendix}
